# Supplementary material for: Turbulent mixing: matching real flows to Kraichnan flows
Source: arXiv:1510.02854 source file (2016-02-04)
Supplement: Supplementary file 1 [file supplemental.pdf]

# Turbulent mixing: matching real flows to Kraichnan flows. Supplemental material

Siim Ainsaar,[1,2] Mihkel Kree,[1] and Jaan Kalda[1]

[1]*Institute of Cybernetics, Tallinn University of Technology*

[2]*Institute of Physics, University of Tartu,*

## 1. DETAILS OF THE SIMULATIONS WITH SINE FLOWS

In our simulations, we are using random velocity field $\boldsymbol{v}$ built as a superposition of incompressible (solenoidal) and irrotational (potential) components: $\boldsymbol{v} = \boldsymbol{v}_\mathrm{s} + \boldsymbol{v}_\mathrm{p}$. In general, the two components may have independent variable magnitudes and correlation times $\tau_\mathrm{s}$ and $\tau_\mathrm{p}$. The solenoidal component $\boldsymbol{v}_\mathrm{s} = (v_{\mathrm{s}x}, v_{\mathrm{s}y})$ is taken of the analytical form

$$\begin{aligned} v_{\mathrm{s}x} &= 1/2\pi \sin(2\pi x)\cos(2\pi y) \\ v_{\mathrm{s}y} &= -1/2\pi \cos(2\pi x)\sin(2\pi y), \end{aligned}$$

where the incompressibility condition $\boldsymbol{\nabla}\cdot\boldsymbol{v}_\mathrm{s} = 0$ holds. After every correlation time $\tau_\mathrm{s}$, the velocity field $\boldsymbol{v}_\mathrm{s}$ is updated by randomly rotating and shifting the $\boldsymbol{v}_s$-field in $xy$-space.

The potential component $\boldsymbol{v}_\mathrm{p} = (v_{\mathrm{p}x}, v_{\mathrm{p}y})$ of the field is taken in the form

$$\begin{aligned} v_{\mathrm{p}x} &= -A_p/2\pi \cos(2\pi x)\sin(2\pi y) \\ v_{\mathrm{p}y} &= -A_p/2\pi \sin(2\pi x)\cos(2\pi y), \end{aligned}$$

where the condition $\boldsymbol{\nabla}\times\boldsymbol{v}_\mathrm{p} = 0$ holds. Note that while we have fixed the magnitude of $\boldsymbol{v}_\mathrm{s}$, the magnitude $A_p$ of $\boldsymbol{v}_\mathrm{p}$ is an adjustable parameter. The field $\boldsymbol{v}_\mathrm{p}$ is randomly updated after every correlation time $\tau_\mathrm{p}$.

The Lyapunov exponents $\lambda_i$ and their diffusivities $\varkappa_i$ are obtained by tracing an ensemble of infinitesimal vector pairs, initially at right angles to each other, in the flow $\boldsymbol{v}(\boldsymbol{x}, t)$. The evolution of an infinitesimal vector $\mathrm{d}\boldsymbol{x}(t)$ is governed by the gradient tensor matrix $\boldsymbol{M}(\boldsymbol{x}, t)$ of $\boldsymbol{v}(\boldsymbol{x}, t)$ as $\frac{\mathrm{d}}{\mathrm{d}t}\mathrm{d}\boldsymbol{x} = \boldsymbol{M}\cdot\mathrm{d}\boldsymbol{x}$, which is solved numerically using 4th order Runge-Kutta method.

We start each realization of the simulation by uniformly placing 1600 vector pairs in the 2D space pointing at random directions while keeping each vector pair at right angles. For calculating each data point of $\lambda_i$ and $\kappa_i$, the statistics is collected over 1000 random realizations of the flow.

In the case of equal correlation times of the two components of the velocity field, the simulation is run up to time $t_\mathrm{max} = \tau_\mathrm{s} = \tau_\mathrm{p}$. In the case of different correlation times ($\tau_\mathrm{s} \neq \tau_\mathrm{p}$), the simulation is run up to an instant $t_\mathrm{max} = n\tau_\mathrm{s} = m\tau_\mathrm{p}$, which is the least common multiplier of the two individual correlation times. Note that since each consecutive application of a new random period of velocity field would act as a multiplicative random process on the infinitesimal vectors, it is sufficient to run the simulation only up to one correlation time (or, correspondingly, the least common multiplier of the two times).

At the end of the simulations, the first Lyapunov exponents $\lambda_1$ and their diffusivities $\kappa_1$ are simply obtained via the average and variance of the logarithms of vector lengths as

$$\begin{aligned} \lambda_i &= \frac{1}{t_\mathrm{max}}\left\langle \ln\left(\frac{|\mathrm{d}\boldsymbol{x}|}{|\mathrm{d}\boldsymbol{x}_0|}\right)\right\rangle, \\ \kappa_i &= \frac{1}{2t_\mathrm{max}}\left[\left\langle \ln^2\left(\frac{|\mathrm{d}\boldsymbol{x}|}{|\mathrm{d}\boldsymbol{x}_0|}\right)\right\rangle - \left\langle \ln\left(\frac{|\mathrm{d}\boldsymbol{x}|}{|\mathrm{d}\boldsymbol{x}_0|}\right)\right\rangle^2\right], \end{aligned}$$

where $|\mathrm{d}\boldsymbol{x}_0|$ is the initial length of the infinitesimal vectors.

The second Lyapunov exponents $\lambda_2$ and their diffusivities $\kappa_2$ are similarly calculated from the heights $\mathrm{d}h$ of parallelograms built from each vector pair.

## 2. CALCULATION OF THE INTEGRALS OF EQUATIONS (3) AND (4)

Our computations are sped up by two integrals:

$$\int_0^{\frac{\pi}{2}} \ln\!\left(p^2\cos^2\alpha + q^2\sin^2\alpha\right)\,\mathrm{d}\alpha = \pi\ln\frac{p+q}{2}, \qquad (1)$$

$$\begin{aligned} &\int_0^{\frac{\pi}{2}} \left[\ln\!\left(p^2\cos^2\alpha + q^2\sin^2\alpha\right)\right]^2\,\mathrm{d}\alpha \\ &\quad = 2\pi\left(\ln\frac{p+q}{2}\right)^2 + \pi\,\mathrm{Li}_2\left[\left(\frac{p-q}{p+q}\right)^2\right], \end{aligned} \qquad (2)$$

where $\mathrm{Li}_2\, x = -\int_0^x [\ln(1-u)]/u\,\mathrm{d}u$ is the dilogarithm, and $p \geq q > 0$. Both integrals are derived in a similar manner, the outline of this is as follows.

Upon denoting $y = \frac{p}{q}$ and $z = \mathrm{e}^{i\alpha}$, the integrals can be written as

$$-\frac{i}{4}\oint f_\xi(z)\,\mathrm{d}z \equiv -\frac{i}{4}\oint_{|z|=1}\left\{\mathrm{Ln}\!\left[A(z^2+z^{-2})+B\right]\right\}^\xi\frac{\mathrm{d}z}{z} \qquad (3)$$

with Ln being the principal branch of the complex logarithm (with the branch cut along the negative real numbers), the constant $A = \frac{y^4-1}{4y^2}$ and $B = \frac{y^4+1}{2y^2}$; $\xi = 1$ corresponds to Eq. (1) and $\xi = 2$ — to Eq. (2). Additionally, define $C = \sqrt{\frac{y^2-1}{y^2+1}}$. By Cauchy's integral theorem, the contour can then be contracted into the shape depicted and labelled in the figure 1.

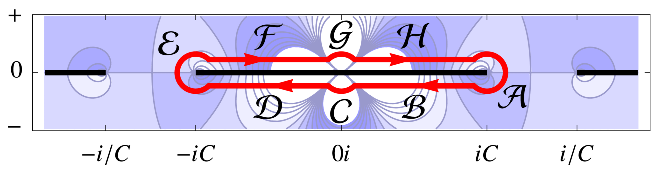


FIG. 1. The integration contour used for the integrals (1) and (2). On the background, we depict $\operatorname{Re} f_2(z)$ from eq. (3). The thick black lines are the branch cuts.

The integrals along the arcs $\mathcal{A}$ and $\mathcal{E}$ tend to zero together with the arcs' radii: if the radius is an infinitesimal $r$, then

$$\int_{\mathcal{A}} f_1(z)\,\mathrm{d}z \sim -\frac{2\pi i r}{C} \to 0, \tag{4}$$

$$\int_{\mathcal{A}} f_2(z)\,\mathrm{d}z \sim -\frac{4\pi i r}{C}\left\{\ln\left[2A\left(\frac{1}{C^3}-C\right)r\right]-1\right\} \to 0, \tag{5}$$

and by symmetry, $\int_{\mathcal{E}} = -\left(\int_{\mathcal{A}}\right)^*$.

On the other hand, the radii of the central arcs $\mathcal{C}$ and $\mathcal{G}$ must be kept finite ($\varrho$), because the integrals (taken separately) would diverge otherwise. As the branch cut of Ln has a height of $2\pi i$, we can approximate (for $x > 0$ and infinitesimal $\varepsilon > 0$)

$$f_1(ix+\varepsilon) - f_1(ix-\varepsilon) \sim \frac{2\pi}{x}, \tag{6}$$

$$f_2(ix+\varepsilon) - f_2(ix-\varepsilon) \sim -4\pi \ln\left[A\left(x^2+\frac{1}{x^2}\right)-B\right]\frac{1}{x}. \tag{7}$$

From these we can calculate

$$\left(\int_{\mathcal{B}} + \int_{\mathcal{H}}\right) f(z)\,\mathrm{d}z = \lim_{\varepsilon\to 0^+}\int_{\varrho}^{C}[f(ix+\varepsilon)-f(ix-\varepsilon)]i\,\mathrm{d}x. \tag{8}$$

Thus we obtain

$$\left(\int_{\mathcal{B}} + \int_{\mathcal{H}}\right) f_1(z)\,\mathrm{d}z = -2\pi i \ln\frac{C}{\varrho}, \tag{9}$$

$$\left(\int_{\mathcal{B}} + \int_{\mathcal{H}}\right) f_2(z)\,\mathrm{d}z = -4\pi i \int_{\varrho}^{C} \ln\left[A(x^2+x^{-2})-B\right]\mathrm{d}x$$
$$= -4\pi i\left[\ln A \ln x - \frac{1}{2}\operatorname{Li}_2\left(C^2x^2\right) - \frac{1}{2}\operatorname{Li}_2\frac{C^2}{x^2} - (\ln x)^2\right]_{x=\varrho}^{C}. \tag{10}$$

Note that $\operatorname{Li}_2 0 = 0$ [allowing us to ignore the infinitesimal term $\operatorname{Li}_2(C^2\varrho^2)$] and $\operatorname{Li}_2 1 = \pi^2/6$. Again by symmetry, $\int_{\mathcal{D}} + \int_{\mathcal{F}} = -\left(\int_{\mathcal{B}} + \int_{\mathcal{H}}\right)^*$.

Finally, the integrals along $\mathcal{C}$ and $\mathcal{G}$ can be calculated for small $\varrho$ using

$$f_\xi\left(\varrho e^{i\varphi}\right) \sim \left(\ln\frac{A}{\varrho^2} + [2\pi i] - 2i\varphi\right)^{\xi}\frac{1}{\varrho e^{i\varphi}}, \tag{11}$$

where the $2\pi i$ must be added only on the arc $\mathcal{C}$, but not on $\mathcal{G}$. If all the integrals along all the paths are added and the outcome simplified, then $\varrho$ cancels out and the results (1) and (2) are obtained.
